# Supplementary material for: Quantum statistical imaging of particles without restriction of the diffraction limit
Source: arXiv:1210.2477 source file (2013-02-21)
Supplement: Supplementary file 1 [file Supplementary.pdf]

# Supplementary: Quantum statistical imaging of two particles without restriction of the diffraction limit

Jin-Ming Cui, Fang-Wen Sun,* Xiang-Dong Chen, Zhao-Jun Gong, and Guang-Can Guo
*Key Laboratory of Quantum Information, University of Science and Technology of China (CAS), Hefei 230026, People's Republic of China*
(Dated: October 8, 2012)

## I. EXPERIMENTAL SETUP

The measurement setup is based on confocal microscopy [1] with Hanbury Brown and Twiss (HBT) detection scheme [2], shown in Figure S1. Polarized 532nm green laser is used to excite NV centers. A numerical aperture of 0.9 objective lens focuses pump laser onto the sample to get the resolution of 400nm. NV fluorescent photons are collected by the same objective lens. After a dichroic mirror and a 600nm long wavelength pass filter, they are coupled to an optical fiber which acts as a confocal pinhole to restrict the corresponding acceptance area with a full width at half maximum (FWHM) of 1$\mu$m. Finally, the fluorescent photons are divided and sent to two avalanche photodiodes (APD) detectors by a fiber beam splitter. Typically for single NV center, each detector has a count rate about 20k/s with 1k/s background noise, including the APD dark count rate of 100/s, with a pumping power of 500$\mu$w. To get confocal scanning images, a three-dimensional closed loop piezo-electric transition stage (Physik Instrumente, P-611.3SF) with a resolution of 1nm is used to scan samples in $x-y$ focusing plane.

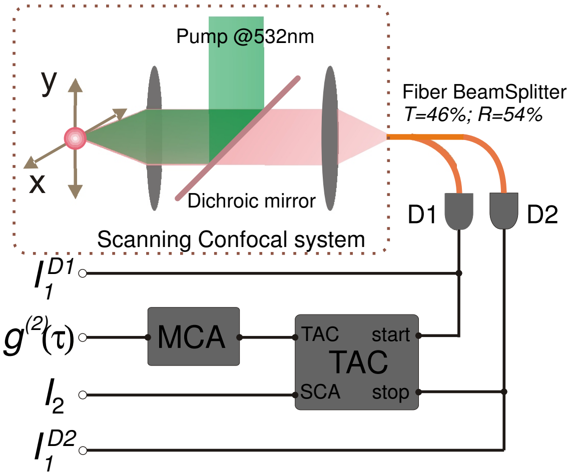


Figure S1: Schematic of measurement setup. Confocal NV fluorescent photons are splitted by a fiber beam splitter with splitting ratio of 46:54 and sent to single photon detector D1, D2. TAC is used to get coincidence counts of D1 and D2 from SCA output, while TAC output is connected to a MCA to implement HBT measurement. $I_1^{D1}$, $I_1^{D2}$, and $I_2$ are count rates of D1, D2 and coincidence rate, respectively.

Coincident rate $I_2$ and second order correlation function $g^{(2)}(\tau)$ [2] are measured with the HBT scheme. A 3m mutimode fibers are inserted between APDs and the fiber beam splitter to shift cross talk peaks far from $\tau = 0$. Fiber modes and electronics independently introduce timing jitters, leading to a spreading of $\tau$ with a FWHM of 1ns. A time-amplitude converter (TAC) with single-channel analyzer (SCA) (Ortect mode 567) records coincident events of two APDs. TAC output signals are statistically analyzed by a multi-channel analyzer (MCA) to get none normalized $G^{(2)}(\tau)$ as long as the lifetime of NV centers $\tau_0$ is much smaller than the mean time between detection events. $g^{(2)}(\tau)$ can be obtained by normalizing $G^{(2)}(\tau)$ with $I_1^{D1} I_1^{D2} t_{bin} T_{int}$, where $I_1^{D1}$ and $I_1^{D2}$ are the two APD count rates, $t_{bin}$ is the time bin width of each channel, and $T_{int}$ is the total integration time. To get the coincident counts rate $I_2$ which equals to $\int_{-t_w/2}^{t_w/2} G^{(2)}(\tau)\, d\tau / T_{int}$, a small SCA window width $t_w$ is set at $\tau = 0$ and coincident events falling in the SCA window are recorded by a counter.

## II. DATA MEASUREMENT

Figure S2 (a) shows a scanning image of 10$\mu$m $\times$ 10$\mu$m square on the surface of diamond. The point ($S_1$) at the center is a two-NV-center pair, corresponding to the second pair with shorter distance demonstrated in the Main Text. The counting rate is about 35k/s. Other darker points whose count rates below 25k/s are single NV centers, such as $S_2$. Second order correlation measurement with $g^{(2)}(0) = 0.55$ in Figure S2(b) confirms two points in the center spot. Here in Figure S2 (b) $g^{(2)}(\tau) > 1$ is caused by metastable shelving state [3]. Figure S2 (c) shows the fluorescent spectrum of the two-NV-center pair with the spectrum resolution of 0.3nm. The zero phonon line at 637nm for NV center is clearly visible, and additional phonon contributions result in the characteristic spectral shape with an overall width of about 120nm [1, 4].

*Electronic address: fwsun@ustc.edu.cn

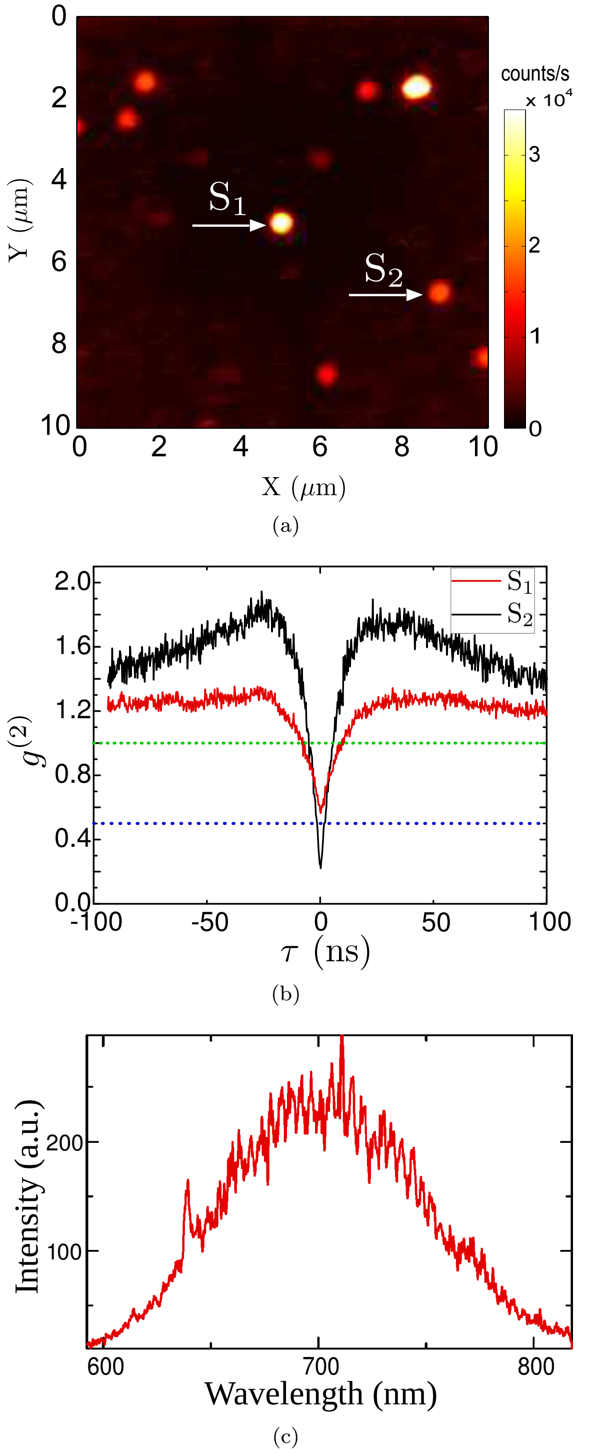


Figure S2: (a) Confocal scanning on the surface of sample. The bright spot ($S_1$) at the center has two NV centers, leading to a count rate about 35 k/s. Other darker spots are single-NV-centers with the counts below 25 k/s, such as $S_2$. (b) Second order correlation function $g^{(2)}(\tau)$ for single-NV-center $S_1$ (Black curve) and two-NV-center pair $S_2$ (Red curve) in (a). The data are not corrected for background photoluminescence. (c) The spectrum of the two-NV-center pair ($S_1$) with a resolution of 0.3 nm.

## III. DATA CORRECTION

In Figure S2 (c), the extra 0.2 background for $g^{(2)}(0)$ of single NV center ($S_2$) is caused by noise and jitter. Noise subtraction and deterministic deconvolution can be done to correct the data to a low background. Taking the noise as Poisson background, we eliminate it with $\epsilon_n = 2s + s^2$, where $s$ is noise to signal ratio, $2s$ and $s^2$ are noise-signal and noise-noise coincidence rates respectively. Therefore the corrected $G_c^{(2)}(\tau)$ is

$$G_c^{(2)}(\tau) = G^{(2)}(\tau) - \epsilon_n \cdot I_{1s}^{D1} I_{1s}^{D2} t_{bin} T_{int}, \tag{S1}$$

where $I_{1s}^{D1}$ and $I_{1s}^{D2}$ are signal count rates obtained by subtracting background noise for D1 and D2 respectively. Renormalization of $G^{(2)}(\tau)$ leads to $g_c^{(2)}(\tau) = 1 + (1+s)^2 \cdot (g^{(2)}(\tau) - 1)$. Subtracting the background noise base, $g_c^{(2)}(0)$ can be reduced to about 0.1.

In the scanning image measurement of $I_2$, a proper SCA detection window $t_w$ should be selected for a compromise between detection rates and precision. Typically $t_w$ is set 2ns, as $g^{(2)}(\tau)$ has a width about 20 ns from Figure S2 (b). In this case, window convolution effect near $\tau = 0$ should be taken into further correction for $I_2$. Combining the noise correction in Eq. S1, correction for $I_{2c}$ is

$$I_{2c} = I_2 - \epsilon_n \cdot I_{1s}^{D1} I_{1s}^{D2} t_w - \epsilon_w \cdot (I_1^{D1} I_1^{D2} t_w - I_2), \tag{S2}$$

where $\epsilon_w$ is SCA window convolution error, which depends on $g_c^{(2)}(\tau)$ and $t_w$ by convolution relation. Here $t_w = 2$ns, $\epsilon_w$ is 5 %.

## IV. DATA PROCESSING

Solving the quadratic equation for each pixel, $I_\pm(x, y)$ can be obtained. However, it still need set $I_\pm(x, y)$ as $I_A(x, y)$ or $I_B(x, y)$. As $I_+ = \max\{I_A, I_B\}$, $I_- = \min\{I_A, I_B\}$, there are two different kinds of cases. For case $I_A(x, y) < I_B(x, y)$ at all pixels, such as the second pair in the Main Text, we can easily set $I_A(x, y) = I_-(x, y)$, $I_B(x, y) = I_+(x, y)$. For the other case, such as the first pair in the Main Text, some pixels meet condition of $I_A < I_B$, and other pixels $I_A > I_B$. In this case there must be positions as $\{x_0, y_0\}$ with $I_A(x_0, y_0) = I_B(x_0, y_0)$, which means the cross-line of two peaks. On one side of cross-line $\{x_0, y_0\}$, $I_A(x, y) = I_-(x, y)$, $I_B(x, y) = I_+(x, y)$; on the opposite side $I_A(x, y) = I_+(x, y)$, $I_B(x, y) = I_+(x, y)$. Theoretically for two single NVs $g_c^2(0)$ can reach 0.5 only when $I_A = I_B$. If it exists, we split $I_\pm(x, y)$ to $I_{A,B}(x, y)$ from the line, else directly set $I_\pm(x, y)$ as $I_{A,B}(x, y)$.

## V. MEASUREMENT RESOLUTION

Because of the low photon collection efficiency, the measurement time for each point is about 200$s$. There are two types of error (resolution) in experiment (Here, we used the data of NV A in second pair.):

(a) Photon counting: Low coincidence count number of $n_2$ is the main restriction. In experiment, there are $10^5$ coincidence events in Fig. 2, inducing the error (resolution) of 0.9nm.

(b) Mechanical error of setup: The piezo translation we used (PI) has a repeat resolution below 10nm. To overcome the repeat error in piezo movement, we divided the measurement to many frames. In the measurement, we got the images in 200 frames by counting 2s for each pixel. Then stack these frames. By this method, the repeat error can be decrease to $10/\sqrt{200} = 0.7$nm. It can be improved with high stable stage. Mechanical drift can be neglected for the measure time is short in this measurement.

If these two errors are independent, total error is about 1.1nm for single $x$ or $y$ axis, which is consistent with resolution (variance) of the direct fitting of $I_A$.

For NV B, the error is about 1.4nm on single axis because of lower photon counts. Then, the total error for the distance is about 2.4nm.


[1] A. Gruber, A. Dräbenstedt, C. Tietz, L. Fleury, J. Wrachtrup, and C. von Borczyskowski, *Science* **276,** 2012 (1997).

[2] Hanbury Brown, R. & Twiss, R. Q. Correlation between photons in two coherent beams of light. *Nature* **177,** 27-29 (1956).

[3] Kurtsiefer, C., Mayer, S., Zarda, P., & Weinfurter, H. Stable solid-state source of single photons. *Phys. Rev. Lett.* **85,** 290-293 (2000).

[4] The Properties of Natural and Synthetic Diamond, edited by J. E. Field (Academic Press, London, 1992).
